# Supplementary material for: A Dynamical Simulation Model of a Cement Clinker Rotary Kiln
Source: arXiv:2405.03200 source file (2024-05-06)
Supplement: Supplementary file 1 [file Appendix.tex]

\section{Appendix - Termodynamic Base functions}
The function $H(T,P,n)$ is used to describe the enthalpy, as it is linear wrt. moles $n$, the mole input can be replace with concentration or flux to obtain enthalpy density and enthalpy flux respectively.
\begin{align}
    H(T,P,n)& = \sum_i n_ih_i(T,P)\\
    h_i(T,P) &= h_i(T_0,P_0) + \int_{T_0}^{T}c_{m,i}(T)dT
\end{align}
$h_i(T,P)$ is the molar enthalpy of composite $i$, with $h_i(T_0,P_0)$ being a reference value, and $c_{m,i}$ is the molar heat capacity as a function of temperature.

The function $V(T,P,n)$ is used to describe the volume, as it is linear wrt. moles $n$, the volume density can be defined by using concentration instead of mole.
\begin{align}
    V(T,P,n) = \sum_i n_i\frac{M_i}{\rho_i(T,P)}
\end{align}
where $M_i$ is the molar mass, and $\rho$ is the density. For solid the composite density is constant, while for gasses the density is given by
\begin{align}
    \rho_i(T_g,P_g) = \frac{M_iP_g}{RT_g}
\end{align}
while assuming ideal gasses.
\section{Appendix - how to compute bed height}
When knowing the temperature, pressure and concentration profile, the volume of the solids is given by:
\begin{align}
    V_k &= 2\pi r_k^2\\
    \hat{V}_s &= V(T_s,P_s,C_s)\\
    V_s &= \hat{V}_sV_k
\end{align}
The corresponding cross-sections of the solid volumes between segments are then computed by:
\begin{align}    
    A_{s,k+\frac{1}{2}} = \pdv{V_{s,k+\frac{1}{2}}}{z} \approx \frac{V_{s,k+1}-V_{s,k}}{\Delta z}
\end{align}
and for the boundary cross-sections, by utilizing the integral relation:
\begin{align}
    V_{s,k} &= \int^{z_{k+\frac{1}{2}}}_{z_{k-\frac{1}{2}}}A_{s,z}dz\approx \frac{A_{s,k-\frac{1}{2}}+A_{s,k+\frac{1}{2}}}{2}\Delta z\\
    A_{s,\frac{1}{2}}  &= \frac{2V_{s,1}}{\Delta z} - A_{s,\frac{3}{2}},\quad 
    A_{s,N_z+\frac{1}{2}} = \frac{2V_{s,N_z}}{\Delta z}  - A_{s,N_z-\frac{1}{2}}
\end{align}
assuming first-order change in the cross area.\\
The fill angle $\theta$ is then computed by solving the equation:
\begin{align}
        A_{s,k} = \frac{r_k^2}{2}(\theta - sin(\theta))
\end{align}
The bed height is then computed by
\begin{align}
    h_{b} = r_k\bigg(1 - \sqrt{cos^2\bigg(\frac{\theta}{2}\bigg)}\bigg)\\
\end{align}
with the cord and slope angle computed from  the bed height:
\begin{align}
    L_{c} &= 2r_k sin\bigg(\frac{\theta}{2}\bigg)\\    
    \phi &= atan\bigg(\pdv{h_{b}}{z}\bigg)
\end{align}

\section{reaction rate of $2H_2 + O_2 = 2H_2O$}
We are interrested in the reaction rate of
\begin{align}
   r_0: 2H_2 + O_2 = 2H_2O
\end{align}
but the reaction is actually
\begin{align}
   r_1:& H_2 + O_2 = H_2O + O \\
   r_2:& H_2 + O = OH+H\\
   r_3:& OH+H + M = H_2O + M
\end{align}
M being a catalysator component.

\begin{align}
   r_1:& k= 2.5*10^{13} (T/298.15)^{0.51} exp(35540/T) [ mol/cm^3s]\cite{Karkach1999}\\
   r_2:& k = exp(14.04) T^(2.270) exp(3501/T) [ mol/cm^3s]\cite{Varga2016}\\
   r_3:& k = exp(55.66) T^(-2.538) exp(-60.79/T) [ mol/cm^3s]\cite{Varga2016}
\end{align}

the combined reactions are
\begin{align}
    \pdv{H_2}{t} = -r_1-r_2,\quad \pdv{H}{t} = r_2-r_3\\
    \pdv{O_2}{t} = -r_1,\quad \pdv{O}{t} = r_1-r_2\\
    \pdv{H_2O}{t} = r_1+r_3,\quad \pdv{OH}{t} = r_2-r_3
\end{align}

the overall reaction rate is then

\begin{align}
    r_0 &= -\frac{1}{2}\pdv{H_2}{t}= -\pdv{O_2}{t} =  \frac{1}{2}\pdv{H_2O}{t}\\
    &= \frac{r_1+r_2}{2}= r_1 =  \frac{r_1+r_3}{2}\\
    &= r_1 = r_2 = r_3
\end{align}

the overall reaction can then be described by the reaction of the first step.

Some of the other reactions can also be written using free radicals
\begin{align}
        \text{$r_{11}$: }& & H_2+O_2&\rightarrow H_2O + O\\
    \text{$r_{12}$: }& & H_2+O &\rightarrow H_2O\\ 
    \text{$r_6$: }& &C + O_2 &\rightarrow CO + O\\
    \text{$r_{10}$: }& & CO + O_2 &\rightarrow CO_2 + O
\end{align}

\section{Algorithm}
The model can be written collectively as
\begin{align}
    \partial_tx& = f(x,y),\quad x=[C;\hat U]\\
    0 &= g(x,y),\quad y=[T;P]
\end{align}
which combine the thermodynamics, geometry, transportation, kinetics into the balance equations (f) and the algebraic equations (g).
Writing them discretely using Euler's (implicit) method gives:
\begin{align}
    x_{n} &= x_{n-1} + f(x_n,y_n)\Delta t\\
    0 &= g(x_{n},y_{n})
\end{align}
The correct "next-step" $x_{n+1}$ and $y_{n+1}$ is then computed by numerical-iteration of the above equations using Newton's method.

initial guess, explicit euler: $x_{n,0} = x_{n-1} + f(x_n-1,y_n-1)\Delta t$ and $y_{n,0} = y_{n-1}$

\begin{align}
    \begin{bmatrix}I- \pdv{f(x_n,y_n)}{x_{n+1}}\Delta t & - \pdv{f(x_n,y_n)}{y_{n+1}}\Delta t\\
    \pdv{g(x_{n+1},y_{n+1})}{x_{n+1}} & \pdv{g(x_{n+1},y_{n+1})}{y_{n+1}}\end{bmatrix}&\begin{bmatrix}\Delta x\\ \Delta y\end{bmatrix} = \begin{bmatrix}x_{n+1} - x_{n} - f(x_n,y_n)\Delta t\\
    g(x_{n+1},y_{n+1})\end{bmatrix}\\
    \begin{bmatrix}
        x_{n+1,i+1}\\y_{n+1,i+1} 
    \end{bmatrix} = &  \begin{bmatrix}
        x_{n+1,i}\\y_{n+1,i} 
    \end{bmatrix} - \begin{bmatrix}\Delta x\\ \Delta y\end{bmatrix} 
\end{align}

\begin{align}
    \pdv{f(x_{n,i})}{x_{n,i}} = \frac{f(x_{n,i}) - f(x_{n-1})}{x_{n,i} - x_{n-1}}
\end{align}
"THIS SECTIONS NEEDS MORE WORK - JAN"

\section{input output}
Kiln: 
$\omega = 0.06 s$ 
$ psi = 0.035 rad$
$ L=51, r=3.95/2, $
$vg0 = 9.0459 m/s$
material load in outlet gas?: $0.24 kg/kg$
pressure loss 100 Pa

onecalc - each part of the kiln has inlet molar flow
need to find the order of compartments
Stream 1 - 11
inlet zone reactor
gas outlet reactor
burning zone reactor
